# Supplementary material for: Strategic Apple Tasting
Source: arXiv:2306.06250 source file (2023-10-28)
Supplement: Supplementary file 1 [file ols_bandit_appendix.tex]

\section{OLS with bandit feedback}
%
\iffalse
\begin{algorithm}[t]
        \SetAlgoNoLine
        \SetAlgoNoEnd
        Assign action $1$ for the first $d$ rounds and action $0$ for the next $d$ rounds\\
        Set $\pv{S}{1}_{2d+1} = \{(\vx_s, \pv{r}{1}_s\}_{s=1}^d$, $\pv{S}{0}_{2d+1} = \{(\vx_s, \pv{r}{0}_s)\}_{s=d+1}^{2d}$\\
        \For{$t = 2d+1, \ldots, T$}
        {   
            Estimate $\pv{\vtheta}{1}$, $\pv{\vtheta}{0}$ as $\pv{\widehat \vtheta}{1}_t$, $\pv{\widehat \vtheta}{0}_t$ using OLS and data $S_t$\\
            Let $\widehat \vbeta_t := \pv{\widehat \vtheta}{1}_t - \pv{\widehat \vtheta}{0}_t$\\
            Assign action $a_t = 1$ if $\langle \widehat \vbeta_t, \vx_t' \rangle \geq \delta \cdot \|\widehat \vbeta_t\|_2$\\
            %
            \uIf{$\langle \widehat \vbeta_t, \vx_t' \rangle \leq 0$}{
                Conclude that $\vx_t' = \vx_t$\\
                %
                $\pv{S}{0}_{t+1} = \pv{S}{0}_t \cup \{(\vx_t, \pv{r}{0}_t)\}$\\
                $\pv{S}{1}_{t+1} = \pv{S}{1}_t$
              }
              \uElseIf{$\langle \widehat \vbeta_t, \vx_t' \rangle > \delta \| \widehat \vbeta_t \|_2$}{
                Conclude that $\vx_t' = \vx_t$\\
                %
                $\pv{S}{1}_{t+1} = \pv{S}{1}_t \cup \{(\vx_t, \pv{r}{1}_t)\}$\\
                $\pv{S}{0}_{t+1} = \pv{S}{0}_t$
              }
              \Else{
                $\pv{S}{1}_{t+1} = \pv{S}{1}_t$\\
                $\pv{S}{0}_{t+1} = \pv{S}{0}_t$
              }
        }
        \caption{Strategy-Aware OLS with Bandit Feedback (\texttt{SA-OLS-B})}
        \label{alg:ols-non-strat-bandit}
\end{algorithm}
\fi

\begin{lemma}
    Under Assumption \khcomment{[]}, $\vx_t' = \vx_t$ if $\langle \pv{\widehat \vtheta}{1}_t - \pv{\widehat \vtheta}{0}_t, \vx_t' \rangle > \delta \|\pv{\widehat \vtheta}{1}_t - \pv{\widehat \vtheta}{0}_t\|_2$ or $\langle \pv{\widehat \vtheta}{1}_t - \pv{\widehat \vtheta}{0}_t, \vx_t' \rangle < 0$.
\end{lemma}
\begin{proof}
    We begin by analyzing the behavior of agent $t$ on a case-by-case basis.

    \textbf{Case 1:} $\langle \pv{\widehat \vtheta}{1}_t - \pv{\widehat \vtheta}{0}_t, \vx_t \rangle < 0$\\
    Since agent $t$ is constrained to modify their context within a $\ell_2$-ball of radius $\delta$, there exists no feasible modification such that they can receive action $1$ under the current policy. 
    Therefore by Assumption \khcomment{[]}, agent $t$ will not modify their context, so $\vx_t' = \vx_t$.
    
    \textbf{Case 2:} $0 \leq \langle \pv{\widehat \vtheta}{1}_t - \pv{\widehat \vtheta}{0}_t, \vx_t \rangle < \delta \|\pv{\widehat \vtheta}{1}_t - \pv{\widehat \vtheta}{0}_t\|_2$\\
    Agent $t$ can receive action $1$ by modifying their context to $\vx_t' = \vx_t + \delta' \|\pv{\widehat \vtheta}{1}_t - \pv{\widehat \vtheta}{0}_t\|_2$ for some $\delta' \leq \delta$.
    By Assumption \khcomment{[]}, agent $t$ will pick $\delta'$ such that $\langle \pv{\widehat \vtheta}{1}_t - \pv{\widehat \vtheta}{0}_t, \vx_t' \rangle = \delta \|\pv{\widehat \vtheta}{1}_t - \pv{\widehat \vtheta}{0}_t\|_2$.

    \textbf{Case 3:} $\langle \pv{\widehat \vtheta}{1}_t - \pv{\widehat \vtheta}{0}_t, \vx_t \rangle \geq \delta \|\pv{\widehat \vtheta}{1}_t - \pv{\widehat \vtheta}{0}_t\|_2$
    Agent $t$ does not need to modify their context to receive action $1$, so they will not do so according to Assumption \khcomment{[]}.

    By Case 1, we can conclude that $\vx_t' = \vx_t$ if $\langle \pv{\widehat \vtheta}{1}_t - \pv{\widehat \vtheta}{0}_t, \vx_t' \rangle < 0$. 
    Likewise, by Case 3 we can infer that $\vx_t' = \vx_t$ if $\langle \pv{\widehat \vtheta}{1}_t - \pv{\widehat \vtheta}{0}_t, \vx_t \rangle > \delta \|\pv{\widehat \vtheta}{1}_t - \pv{\widehat \vtheta}{0}_t\|_2$.
    However nothing can be said in general about the case where $\langle \pv{\widehat \vtheta}{1}_t - \pv{\widehat \vtheta}{0}_t, \vx_t' \rangle = \delta \|\pv{\widehat \vtheta}{1}_t - \pv{\widehat \vtheta}{0}_t\|_2$, due to Case 2.
\end{proof}
